# Supplementary material for: Efficient Temporally-Aware DeepFake Detection using H.264 Motion Vectors
Source: arXiv:2311.10788 source file (2024-02-22)
Supplement: Supplementary file 1 [file 11_supplementary.tex]

%Ablation study on different merging methods from Alessio could possibly go here:

"We also experimented with stacking the diverse inputs, but this gave us a drop in accuracy of over 13\%. "

% \begin{itemize}
%     \item Image compression: The model should be robust to different video compression levels.
%     \item Gaussian noise: The model should decouple the signal from the noise, e.g. in low-light videos.
%     \item Gaussian blur: The model should be robust to lower quality or out of focus videos.
%     \item RGB and Hue-Saturation-Value shifts: Changing the color distribution (by manipulating each pixel) is used to increase the resistance of the model to lighting biases.
%     \item FancyPCA: First introduced by Krizhevsky et al.~\cite{NIPS2012_c399862d} in their submission for the LSVRC-2010 contest. This captures an important property of natural images, i.e. that the model should be able to detect object identity even if there are changes in the intensity and color of the illumination.
%     \item Random Brightness Contrast: Allows for the network to learn different illuminations/contrasts for one scene.
%     \item Grey-scale: Sometimes, videos are transformed to grey-scale and the model should also learn to be efficient in this context.
% \end{itemize}
